# Supplementary material for: Undulatory swimming in viscoelastic fluids
Source: arXiv:1102.3894 source file (2011-05-13)
Supplement: Supplementary file 1 [file SupplementaryMaterial_FINAL.pdf]

# Supplementary Material

April 8, 2011

## Fluid Rheology

### Shear Viscosity Curves

We use a stress-controlled cone-plate rheometer to characterize the carboxy-methyl cellulose (CMC) and xanthan gum (XG) solutions. The viscosity curves are shown in Fig. 1. Note that the mixture of low molecular weight Halocarbon oils show constant shear viscosity and are not shown. The XG solution shows significant shear-rate dependent viscosity while only the more concentrated CMC solutions show shear-thinning effects. We quantify these effects by computing the power law index $n$ (see Table 1). The power law index for XG is 0.35.

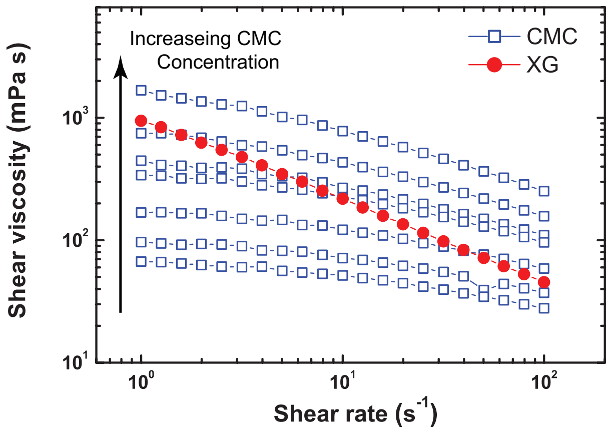


Figure 1: Viscosity curves for both CMC and XG solutions. The CMC concentration in solution ranges from 1000 ppm to 8000 ppm by weight (from bottom to top in the plot). Solid circles represent the 3000 ppm aqueous solution of xanthan gum. The values of the power law index $n$ are 0.65 and 0.35 for the 8000 ppm CMC and the xanthan gum solutions, respectively.

### Fluid Relaxation Times

Fluid relaxation times are obtained by fitting the stress relaxation data (Fig. 2) with the generalized linear viscoelastic model of a single relaxation time of the type $G(t) = G_0 e^{-t/\lambda}$,

| c (ppm) | $n$ |
|---|---|
| 1500 | 0.83 |
| 2000 | 0.81 |
| 3000 | 0.80 |
| 4500 | 0.76 |
| 5000 | 0.74 |
| 6000 | 0.70 |
| 8000 | 0.65 |

Table 1: The values of the power law indexes $n$ of the various CMC solutions used in this work.

where $G(t)$ is the fluid shear modulus and $\lambda$ is the longest fluid relaxation time. Figure 2 shows the data and a sample fitting. The relaxation times of CMC fluids are given in Table 2.

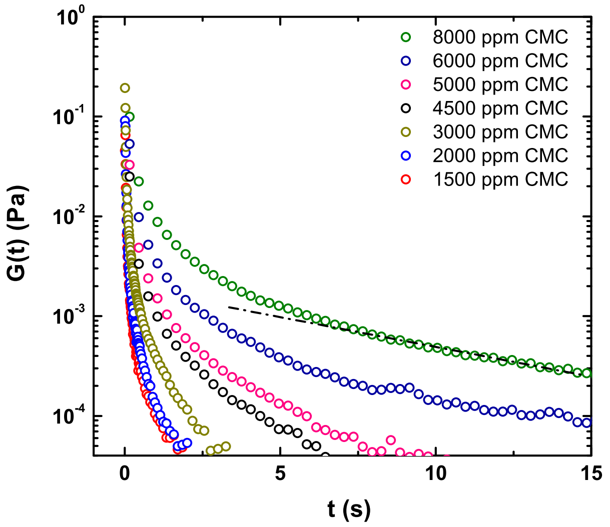


Figure 2: Stress relaxation data for the CMC fluids. The data is fitted to a linear viscoelastic model (dashed line).

| c (ppm) | $\lambda$ (s) |
|---|---|
| 1500 | 0.4 |
| 2000 | 0.6 |
| 3000 | 0.8 |
| 4500 | 2.1 |
| 5000 | 2.3 |
| 6000 | 3.4 |
| 8000 | 5.6 |

Table 2: Relaxation times of the CMC solutions.

## Experimental Methods: imaging the nematode *C. elegans*

We measured a minimum of 12 and a maximum of 18 nematodes for each experiment for an average of 15 nematodes per experiment. The relative standard deviation of nematode's kinematics, i.e. the swimming speed, bending wave speed, beating frequency and amplitude, is less than 15% and the standard error is less than 5%.

The swimming motion of *C. elegans* is imaged using standard bright-field microscopy (1024 x 1024 pixels). The depth of focus of the objective (Apochromat 5x/0.16) is 30 $\mu$m. The focal plane is set on the longitudinal axis of the nematode body. The nematode beats primarily in the observation plane during the recordings, and the amplitude of the out-of-plane beatings is less than 6% amplitude of planar beatings.

## Reynolds number definition

The Reynolds number is defined as $Re = \rho U L/\mu_{\text{eff}}$, where $\mu_{\text{eff}}$ is an effective viscosity calculated from the viscosity data averaged between the shear-rate values ranging from 10 to 20 $\text{s}^{-1}$. This range of shear-rates corresponds to the characteristic shear-rates of the measured flow fields. $U$ and $L$ are the swimming speed and length of the nematode, respectively. $\rho$ is the density of the fluid.
